# Supplementary material for: Anomaly Detection based on Markov Data: A Statistical Depth Approach
Source: arXiv:2406.16759 source file (2025-02-26)
Supplement: Supplementary file 1 [file norm_unbounded_markov_path.tex]

Notice that \(\{||\chain||_\infty<\infty\}\) can be written as
\(\cup_{n=1}^{\infty}{\{||\chain||_\infty\leq n\}}\). Moreover,
\begin{equation*}
    \{||\chain||_\infty\leq n\} =\left\{\max_{i}||X_i||\leq n\right\}=\bigcap_{i=0}^{\infty}\left\{||X_i||\leq n\right\}=\left(\bigcup_{i=0}^{\infty}\{||X_i||>n\}\right)^c \subset\{||X_i||\in C_n \;\;\textnormal{i.o.}\}^c.
\end{equation*}
The Harris recurrence of the chain implies that \(\P(||X_i||\in C_n
\;\;\textnormal{i.o.})=1\), hence, \(\P(||\chain||_\infty\leq n)=1\). The first part of the proposition
now follows from the union bound.
